# Supplementary material for: Anatomy of the ATLAS diboson anomaly
Source: arXiv:1507.01638 ancillary file (2015-09-04)
Supplement: Supplementary file 1 [file likelihood.pdf]

```

(* Joint likelihood of measuring nWW,
nWZ and nZZ excess events at 2 TeV ignoring background uncertainties. *)

(* Observed number of events in each channel over 3 mass bins around 2 TeV *)
obs1 = {2, 6, 5, 0, 4, 0};
obs2 = {1, 7, 5, 0, 3, 1};
obs3 = {0, 8, 5, 0, 2, 2};
(* Expected number of SM events in
each channel over 3 mass bins around 2 TeV *)
backgroundexp = {2.0908, 2.7192, 1., 2.43, 0.4608, 0.3392};
(* Efficiency to get a fat jet from hadronically decaying boson *)
epsilon = 0.33 × 0.67;
(* Matrix of probabilities for tagging a certain diboson signal region*)
M = {{0.063, 0.182, 0.132, 0.018, 0.025, 0.001},
{0.028, 0.139, 0.143, 0.057, 0.090, 0.007},
{0.012, 0.087, 0.155, 0.047, 0.165, 0.044}};
(* Number of delta chi^2 to go up for 70% CL *)
d70cl = 3.67;
d95cl = 7.82;

(* Given signal event rates sWW,sWZ,
sZZ in the WW,WZ and ZZ channels respectively,
give the number of expected tagged events in each signal region *)
tottag[sWW_, sWZ_, sZZ_] := backgroundexp + epsilon {0.45 sWW, 0.47 sWZ, 0.49 sZZ}.M
(*convert disjoint sig regs into ww,wz and zz*)
toATLAS[a_, b_, c_, d_, e_, f_] := {a+b+c, b+c+d+e, c+e+f}
(* Poisson probability of obtaining n events on a background of mu *)
poiss[n_, mu_] := Exp[-mu] mu^n / n!
(* Joint likelihood for obtaining nWW,nWZ,nZZ events tagged in the WW,
WZ and ZZ signal regions, respectively *)
likelihood[obsvec_, sWW_, sWZ_, sZZ_] := Module[{expvec},
expvec = tottag[sWW_, sWZ_, sZZ];
Apply[Times, poiss[#[[1]], #[[2]]] & /@ Transpose[{obsvec, expvec}]]
]
totallikelihood[sWW_, sWZ_, sZZ_] := likelihood[obs1, sWW, sWZ, sZZ] +
likelihood[obs2, sWW, sWZ, sZZ] + likelihood[obs3, sWW, sWZ, sZZ]

```

```

(* Calculate the best-fit chi^2 correctly normalised *)
m = NMinimize[{-2 Log[totallikelihood[sWW, sWZ, sZZ]],
  sWW ≥ 0 && sWZ ≥ 0 && sZZ ≥ 0}, {sWW, sWZ, sZZ}]
minchi2 = m[[1]];
allcl70 = minchi2 + d70cl;
allcl95 = minchi2 + d95cl;
lumi = 20.3;
tottag[sWW, sWZ, sZZ] /. m[[2]]
(* These probe the origins of the 3 panels in Fig 3 *)
NMinimize[{-2 Log[totallikelihood[sWW, 0, 0]], sWW ≥ 0}, {sWW}]
tottag[sWW, 0, 0] /. %[[2]]
NMinimize[{-2 Log[totallikelihood[0, sWZ, 0]], sWZ ≥ 0}, {sWZ}]
tottag[0, sWZ, 0] /. %[[2]]
NMinimize[{-2 Log[totallikelihood[0, 0, sZZ]], sZZ ≥ 0}, {sZZ}]
tottag[0, 0, sZZ] /. %[[2]]
Print["Best fit ",  $\chi^2$ , " of three parameter fit=",
  m[[1]], " for point m=", m[[2]], " 2d 70% CL is at ",
   $\chi^2$ , "=", m[[1]] + d70cl, " , 95% is at ", m[[1]] + d95cl]

{20.9324, {sWW → 105.572, sWZ →  $-8.58769 \times 10^{-22}$ , sZZ → 118.029}}
{2.90599, 5.74338, 4.36851, 3.22006, 2.83327, 0.912337}
{24.1248, {sWW → 253.854}}
{3.682, 7.31601, 4.33395, 2.88463, 1.09223, 0.364457}
{21.706, {sWZ → 223.644}}
{2.74153, 5.94962, 4.32338, 3.7547, 2.55244, 0.501883}
{21.7459, {sZZ → 176.782}}
{2.32063, 4.38546, 3.96863, 3.33016, 3.62095, 1.18191}

Best fit  $\chi^2$  of three parameter fit=20.9324
  for point m={sWW → 105.572, sWZ →  $-8.58769 \times 10^{-22}$ , sZZ → 118.029}
  2d 70% CL is at  $\chi^2$ =24.6024, 95% is at 28.7524

```

```

(* Now calculate 2d plots under the assumption that one
   of the channels has zero signal. First assume WW is zero *)
mww0 = NMinimize[{-2 Log[totallikelihood[0., sWZ, sZZ]], sWZ >= 0 && sZZ >= 0},
  {sWZ, sZZ}]
tottag[0, sWZ, sZZ] /. mww0[[2]]
Apply[toATLAS, tottag[0, sWZ, sZZ] /. mww0[[2]]]
minchi2ww0 = mww0[[1]];
ww0cl70 = minchi2ww0 + d70cl
ww0cl95 = minchi2ww0 + d95cl
(* Using luminosity to convert to a cross-section times BR *)
cp1 = ContourPlot[-2 Log[totallikelihood[0., lumi sWZ, lumi sZZ]],
  {sWZ, 0, 25}, {sZZ, 0, 25}, Contours -> {ww0cl70, ww0cl95}];
{21.3779, {sWZ -> 118.708, sZZ -> 86.281}}
{2.54837, 5.24711, 4.21289, 3.57248, 3.11337, 0.836845}
{12.0084, 16.1459, 8.16311}
25.0479
29.1979

```

```

cp1 = Show[cp1, LabelStyle -> {18, GrayLevel[0]},
  FrameLabel -> {" $\sigma(X^\pm) \times \text{BR}(X^\pm \rightarrow W^\pm Z) / \text{fb}$ ", " $\sigma(X^0) \times \text{BR}(X^0 \rightarrow ZZ) / \text{fb}$ "},
  PlotLabel -> "No WW Signal"];
Show[cp1, Graphics[{White, PointSize[0.03], Point[{sWZ / lumi, sZZ / lumi}]}]] /.
  mww0[[2]] /.
  {EdgeForm[], r_? (MemberQ[{RGBColor, Hue, CMYKColor, GrayLevel}, Head[#]] &),
    i___} -> {EdgeForm[r], r, i}
Export["0ww.pdf", %];
tottag[0., sWZ, sZZ] /. mww0[[2]]

```

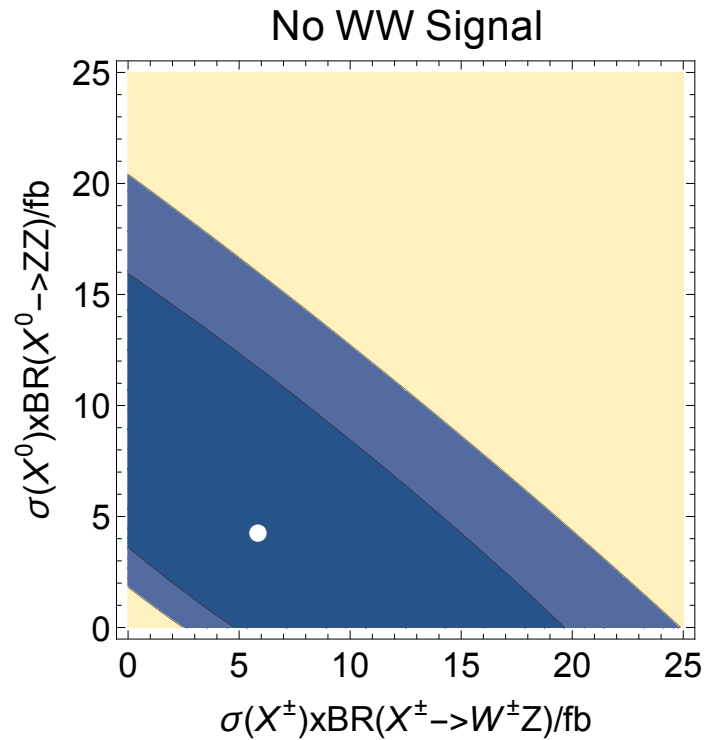

```
{2.54837, 5.24711, 4.21289, 3.57248, 3.11337, 0.836845}
```

```

(* Now assume WZ is zero *)
mwz0 =
  NMinimize[{-2 Log[totallikelihood[sWW, 0., sZZ]], sWW ≥ 0 && sZZ ≥ 0}, {sWW, sZZ}]
minchi2wz0 = mwz0[[1]];
tottag[sWW, 0, sZZ] /. mwz0[[2]]
Apply[toATLAS, tottag[sWW, 0, sZZ] /. mwz0[[2]]]
wz0cl70 = minchi2wz0 + d70cl
wz0cl95 = minchi2wz0 + d95cl
(* Using luminosity to convert to a cross-section times BR *)
cp2 = ContourPlot[-2 Log[totallikelihood[lumi sWW, 0., lumi sZZ]],
  {sWW, 0, 25}, {sZZ, 0, 25}, Contours → {wz0cl70, wz0cl95};
{20.9324, {sWW → 105.572, sZZ → 118.029}}
{2.90599, 5.74338, 4.36851, 3.22006, 2.83327, 0.912337}
{13.0179, 16.1652, 8.11412}
24.6024
28.7524

```

```

cp2 = Show[cp2, LabelStyle -> {18, GrayLevel[0]},
  FrameLabel -> {" $\sigma(X^0) \times \text{BR}(X^0 \rightarrow W^+W^-) / \text{fb}$ ", " $\sigma(X^0) \times \text{BR}(X^0 \rightarrow ZZ) / \text{fb}$ "},
  PlotLabel -> "No WZ Signal"];
cp2 = Show[cp2, Graphics[{White, PointSize[0.03],
  Point[{sWW / lumi, sZZ / lumi}]}] /. mwz0[[2]]];
cp2 /. {EdgeForm[], r_? (MemberQ[{RGBColor, Hue, CMYKColor, GrayLevel},
  Head[#]] &), i___} -> {EdgeForm[r], r, i}
Export["0wz.pdf", %];
tottag[0., sWW, sZZ] /. mwz0[[2]]

```

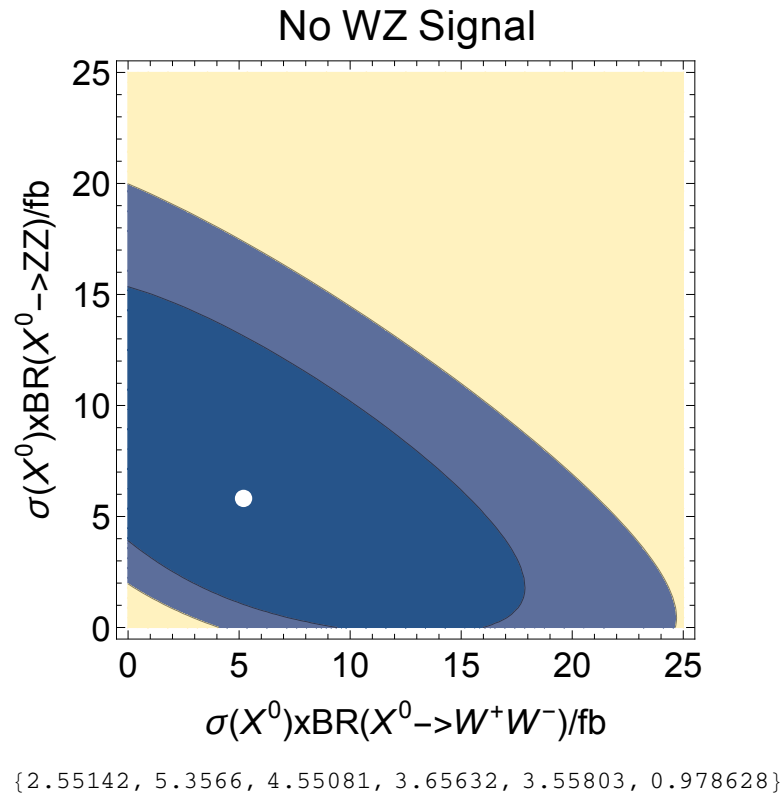

```

(* Now assume ZZ is zero *)
mzz0 =
  NMinimize[{-2 Log[totallikelihood[sWW, sWZ, 0.]], sWW ≥ 0 && sWZ ≥ 0}, {sWW, sWZ}]
tottag[sWW, sWZ, 0] /. mzz0[[2]]
Apply[toATLAS, tottag[sWW, sWZ, 0] /. mzz0[[2]]]
minchi2zz0 = mzz0[[1]];
zz0cl70 = minchi2zz0 + d70cl
zz0cl95 = minchi2zz0 + d95cl
(* Using luminosity to convert to a cross-section times BR *)
cp3 = ContourPlot[-2 Log[totallikelihood[lumi sWW, lumi sWZ, 0.]],
  {sWW, 0, 25}, {sWZ, 0, 25}, Contours → {zz0cl70, zz0cl95}];
{21.706, {sWW → 1.03452, sWZ → 222.83}}
{2.74565, 5.9566, 4.32488, 3.75174, 2.5474, 0.501394}
{13.0271, 16.5806, 7.37367}
25.376
29.526

```

```

cp3 = Show[cp3, LabelStyle -> {18, GrayLevel[0]},
  FrameLabel -> {" $\sigma(X^0) \times \text{BR}(X^0 \rightarrow W^+ W^-) / \text{fb}$ ", " $\sigma(X^\pm) \times \text{BR}(X^\pm \rightarrow W^\pm Z) / \text{fb}$ "},
  PlotLabel -> "No ZZ Signal"];
Show[cp3, Graphics[{{White, PointSize[0.03], Point[{sWW / lumi, sWZ / lumi}]}}]] /.
  mzz0[[2]] /.
  {EdgeForm[], r_? (MemberQ[{RGBColor, Hue, CMYKColor, GrayLevel}, Head[#]] &),
    i___} -> {EdgeForm[r], r, i}
Export["0zz.pdf", %];
tottag[sWW, sWZ, 0] /. mzz0[[2]]

```

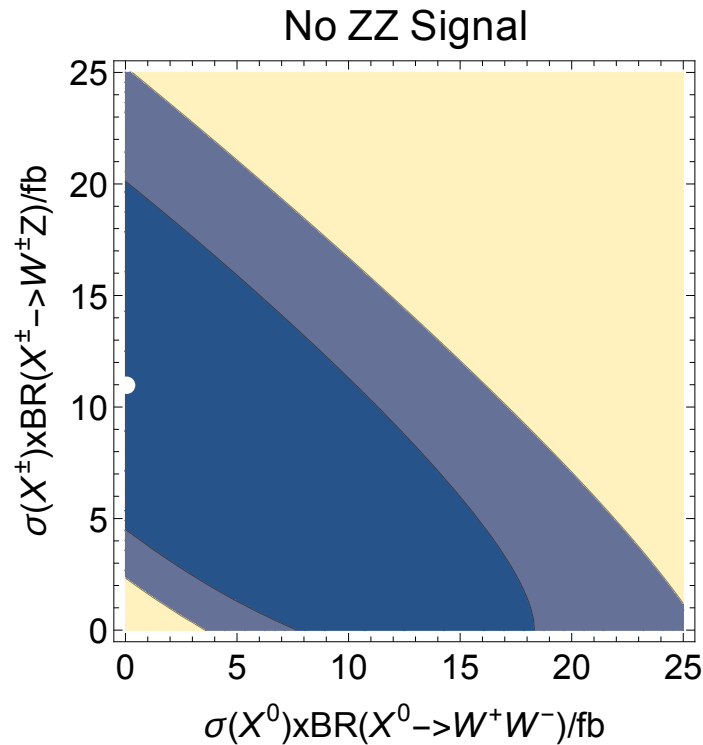

```
{2.74565, 5.9566, 4.32488, 3.75174, 2.5474, 0.501394}
```

(\* Now, we wish to plot 2d likelihood contours not making any assumptions about the signal numbers, allowing them all to vary \*)

```

cp4 = ContourPlot[NMinimize[
  {-2 Log[totallikelihood[lumi sWW, lumi sWZ, lumi sZZ]], sWW >= 0}, {sWW}][[1]],
  {sWZ, 0, 25}, {sZZ, 0, 25}, Contours -> {allc170, allc195}];

```

```

cp4 = Show[cp4, LabelStyle -> {18, GrayLevel[0]},
  FrameLabel -> {" $\sigma(X^\pm) \times \text{BR}(X^\pm \rightarrow W^\pm Z) / \text{fb}$ ", " $\sigma(X^0) \times \text{BR}(X^0 \rightarrow ZZ) / \text{fb}$ "}];
Show[cp4, Graphics[{White, PointSize[0.03], Point[{sWZ / lumi, sZZ / lumi}]}]] /.
  m[[2]] /.
  {EdgeForm[], r_? (MemberQ[{RGBColor, Hue, CMYKColor, GrayLevel}, Head[#]] &),
    i___} -> {EdgeForm[r], r, i}
Export["ww.pdf", %];

```

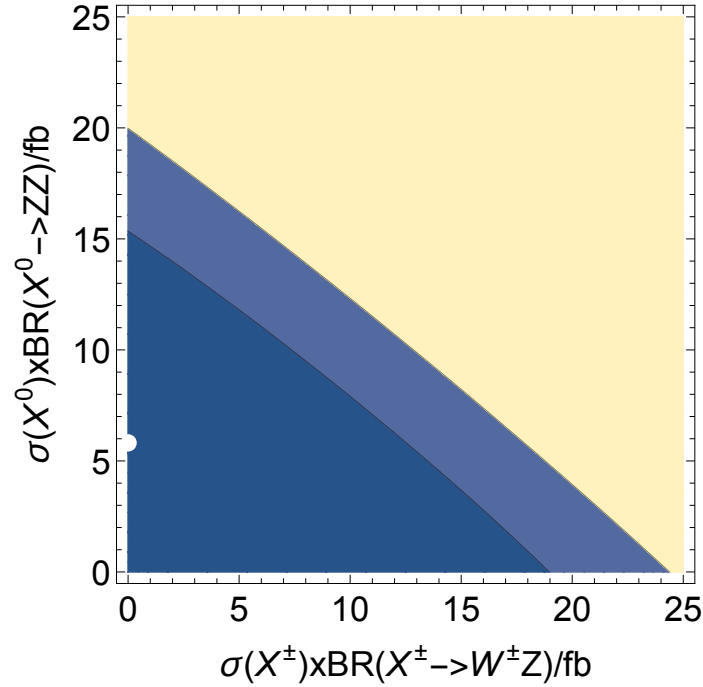

```

cp5 = ContourPlot[
  NMinimize[{-2 Log[totallikelihood[lumi sWW, lumi sWZ, lumi sZZ]], sWZ ≥ 0},
    {sWZ}][[1]], {sWW, 0, 25}, {sZZ, 0, 25},
  Contours -> {allc170, allc195}, LabelStyle -> {18, GrayLevel[0]},
  FrameLabel -> {" $\sigma(X^0) \times \text{BR}(X^0 \rightarrow W^+ W^-) / \text{fb}$ ", " $\sigma(X^0) \times \text{BR}(X^0 \rightarrow ZZ) / \text{fb}$ "}];

```

```
Show[cp5, Graphics[{White, PointSize[0.03], Point[{sWW / lumi, sZZ / lumi}]}]] /.
  m[[2]] /.
  {EdgeForm[], r_? (MemberQ[{RGBColor, Hue, CMYKColor, GrayLevel}, Head[#]] &),
    i___} :> {EdgeForm[r], r, i}
Export["wz.pdf", %];
```

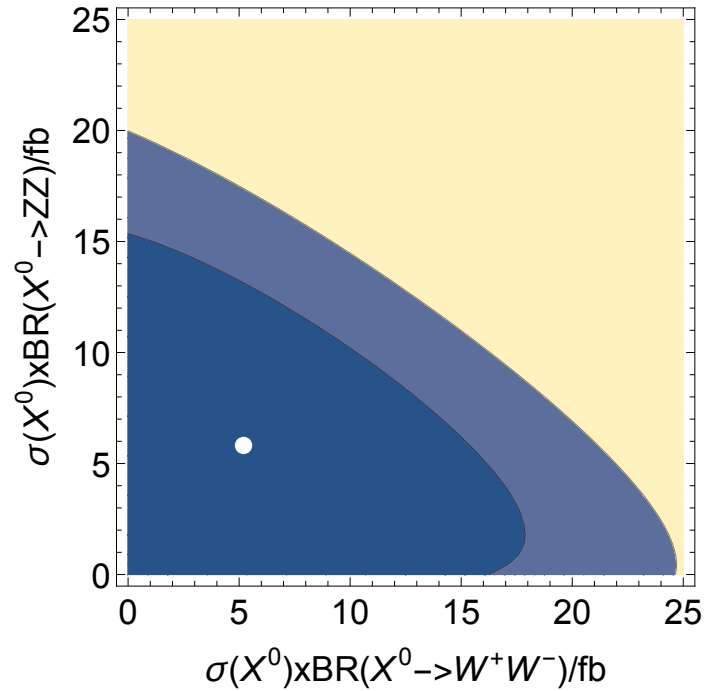

```
cp6 = ContourPlot[
  NMinimize[{-2 Log[totallikelihood[lumi sWW, lumi sWZ, lumi sZZ]], sZZ ≥ 0},
    {sZZ}][[1]], {sWW, 0, 25}, {sWZ, 0, 25},
  Contours → {allc170, allc195}, LabelStyle → {18, GrayLevel[0]},
  FrameLabel → {"σ(X⁰)xBR(X→W⁺W⁻)/fb", "σ(X±)xBR(X±→W±Z)/fb"}];
```

```
Show[cp6, Graphics[{White, PointSize[0.03], Point[{sWW / lumi, sWZ / lumi}]}] /.
  m[[2]] /.
  {EdgeForm[], r_? (MemberQ[{RGBColor, Hue, CMYKColor, GrayLevel}, Head[#]] &),
    i___} => {EdgeForm[r], r, i}
Export["zz.pdf", %];
```

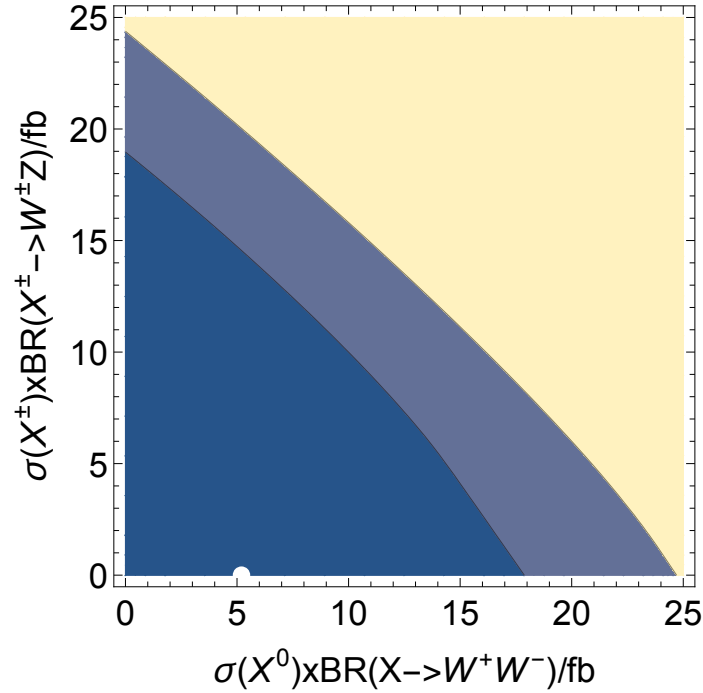

```
Plot[{NMinimize[{-minchi2 - 2 Log[totallikelihood[lumi x, lumi sWZ, lumi sZZ]],
  sWZ ≥ 0 && sZZ ≥ 0}, {sWZ, sZZ}][[1]],
  NMinimize[{-minchi2 - 2 Log[totallikelihood[lumi sWW, lumi x, lumi sZZ]],
  sWW ≥ 0 && sZZ ≥ 0}, {sWW, sZZ}][[1]],
  NMinimize[{-minchi2 - 2 Log[totallikelihood[lumi sWW, lumi sWZ, lumi x]],
  sWW ≥ 0 && sWZ ≥ 0}, {sWW, sWZ}][[1]], d95cl}, {x, 0, 25},
  PlotLegends → {WW, WZ, ZZ, "95% CL"}, LabelStyle → {18, GrayLevel[0]},
  AxesLabel → {"σxBR/fb", Δχ²}]
Export["oneD.pdf", %];
```

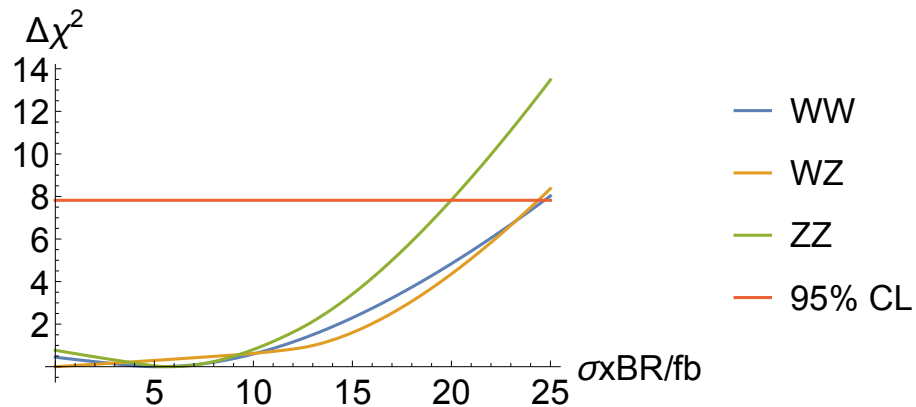

```

NMinimize[{-minchi2 - 2 Log[totallikelihood[lumi 24.7, lumi sWZ, lumi sZZ]],
  sWZ ≥ 0 && sZZ ≥ 0}, {sWZ, sZZ}][[1]]
NMinimize[{-minchi2 - 2 Log[totallikelihood[lumi sWW, lumi 24.4, lumi sZZ]],
  sWW ≥ 0 && sZZ ≥ 0}, {sWW, sZZ}][[1]]
NMinimize[{-minchi2 - 2 Log[totallikelihood[lumi sWW, lumi sWZ, lumi 20]],
  sWW ≥ 0 && sWZ ≥ 0}, {sWW, sWZ}][[1]]
7.81988
7.83386
7.83511

{minchi2ww0, minchi2wz0, minchi2zz0, minchi2}
{21.3779, 20.9324, 21.706, 20.9324}

```
